# Supplementary material for: MarkushGlyph and OCSRGlyph: Improved Chemical Structure Recognition
Source: arXiv:2607.28532 source file (2026-07-30)
Supplement: Supplementary file 1 [file appendix_updates.tex]

% ═══════════════════════════════════════════════════════════════════════════════
% Appendix updates for Experiments 5 (8e/8f) and 6
%
% INSERT LOCATION: Replace the existing "Formal Write-ups" appendix section
% in main.tex with the expanded version below. Also add the v6 references
% to the "Agent Self-Reports" section if applicable.
%
% Compile context: tectonic main.tex (after merging)
% ═══════════════════════════════════════════════════════════════════════════════

% ─── UPDATED FORMAL WRITE-UPS ────────────────────────────────────────────────

\section{Formal Write-ups}

\begin{itemize}
  \item \texttt{paper\_v1.tex} --- Experiment 1: Original warm-start OCSR run (complete, reviewed)
  \item \texttt{paper\_v2.tex} --- Experiment 2: Charter + cold-start reproduction (in progress)
  \item \texttt{paper\_v5.tex} --- Experiment 5: From-scratch OCSR, single-model training campaign (draft; covers Steps 1--8f, error analysis, and stereo-enriched training)
  \item Experiment 6 (behavioral specification, v6) is documented in this lab notebook only --- a formal write-up will follow once the multitask experiment~H trajectory completes and cross-campaign comparison is finalized.
\end{itemize}

\section{Agent Self-Reports}

\begin{itemize}
  \item \texttt{aries\_report.pdf} --- Aries v1 self-report (6 pages, Iter 0--18)
  \item \texttt{aries\_report\_v2.pdf} --- Aries v2 self-report (4 pages, Iter 0--26)
\end{itemize}

% ─── NEW APPENDIX SECTION: V6 BEHAVIORAL DATA ────────────────────────────────

\section{Experiment 6 behavioral data}
\label{app:v6_behavioral}

Table~\ref{tab:v6_monitoring_log} lists all monitoring directives
issued during the v6 campaign, with timestamps and categories.
Each entry corresponds to a scripted-heartbeat check that produced
a non-trivial steering intervention.

\begin{table}[htbp]
\centering
\caption{Monitoring interventions during the v6 campaign.
  Category codes: AUG = augmentation compliance,
  EVAL = evaluation standardization, BUDGET = trajectory-budget
  management.}
\label{tab:v6_monitoring_log}
\small
\begin{tabular}{rlll}
\toprule
\textbf{\#} & \textbf{Category} & \textbf{Context} & \textbf{Directive} \\
\midrule
1 & AUG   & Exp A    & Apply augment\_v2 (18 transforms) \\
2 & AUG   & Exp B    & augment\_v2 still missing; re-apply \\
3 & EVAL  & Exp D    & Run full 5,704-row eval, not partial \\
4 & AUG   & Exp E    & augment\_v2 omitted again \\
5 & EVAL  & Exp E2   & Use canonical EM, not graph-only \\
6 & BUDGET & ---     & Trajectory budget expired; restart \\
7 & BUDGET & ---     & Second trajectory budget expired; restart \\
\bottomrule
\end{tabular}
\end{table}

\section{Cross-campaign comparison}
\label{app:cross_campaign}

Table~\ref{tab:cross_campaign} compares key metrics across all
completed campaigns.

\begin{table}[htbp]
\centering
\caption{Cross-campaign comparison.  ``Experiments'' counts
  distinct training runs.  ``Wall clock'' is approximate elapsed
  time from first to last experiment.  ``Best EM'' is canonical
  exact-match on the 5,704-row USPTO benchmark.  ``Human msg''
  counts human messages sent directly to the agent (excluding
  scripted heartbeat checks).}
\label{tab:cross_campaign}
\small
\begin{tabular}{lccccc}
\toprule
\textbf{Campaign} & \textbf{Experiments} & \textbf{Wall clock} & \textbf{Best EM} & \textbf{Human msg} & \textbf{Primary finding} \\
\midrule
v1 (warm-start)  & 26 iter & ${\sim}$20 h & 0.926$^*$ & 5 & Agent finds post-processing \\
v2 (cold-start)  & 26 iter & ${\sim}$20 h & 0.926$^*$ & 0 & Charter closes autonomy gap \\
v3 (from-scratch) & --- & $<$4 h & --- & --- & Terminated: anchoring failure \\
v4 (from-scratch) & --- & $<$8 h & --- & --- & Terminated: survey gap \\
v5 (from-scratch) & 15 & ${\sim}$5 d & \textbf{0.9104} & 3 & Data ceiling, not capacity \\
v6 (behavioral)   & 14 & ${\sim}$18 h & 0.905 & 0$^\dagger$ & $5$--$7\times$ throughput via spec \\
\bottomrule
\end{tabular}
\smallskip

\noindent $^*$Weighted EM across 4 benchmarks (JPO, CLEF, UOB, USPTO); not directly
comparable to v5/v6 USPTO-only numbers.\\
$^\dagger$Zero direct human messages; 7 scripted heartbeat directives (Table~\ref{tab:v6_monitoring_log}).
\end{table}
