# Supplementary material for: MarkushGlyph and OCSRGlyph: Improved Chemical Structure Recognition
Source: arXiv:2607.28532 source file (2026-07-30)
Supplement: Supplementary file 2 [file appendix_repro_DRAFT.tex]

%% ============================================================================
%% DRAFT reproducibility appendix for the OCSR+Markush paper.
%% NOT wired into the build. Intended to sit alongside the existing
%% \section{Reproducibility} in appendix_b.tex; renumber the label if merged.
%%
%% Every count is verified against an on-cluster manifest or run record, named
%% inline in a trailing % comment. UNVERIFIED / DISCREPANCY items are flagged.
%% ============================================================================

\section{Data Provenance and Reproducibility}
\label{app:repro_data}

This appendix makes the training-data construction auditable. Each mixture is
written with a \texttt{manifest.json} recording its seed, partition counts,
per-source provenance, target-format conversion, and (for the ordinary-molecule
mixes) decontamination results. The manifests live on the cluster under
\path{/data/alex/autoresearch/campaigns/markush/prepared/v5/stable-scaling/}
and \path{/data/alex/autoresearch/campaigns/ocsr/}. All Markush mixes use seed
74; the OCSR model uses recipe seed 42.
% markush manifests: "seed": 74 in every manifest; ocsr seed in v8-3-recipe.json "seed": 42

\subsection{Markush base mixture (250k)}
\label{app:repro_markush_base}

The base mixture is built by \texttt{scripts/build\_stable\_scaling\_sft\_mix.py}
from two prepared partitions and is deterministic given the seed.

\begin{figure}[tbp]
\begin{footnotesize}
\begin{verbatim}
=== Listing: Markush base mixture (no-synthetic-250k-seed74-80base-20hard) ===
Builder: scripts/build_stable_scaling_sft_mix.py   (autoresearch-markush)
Command (from manifest "command" field):
  build_stable_scaling_sft_mix \
    --partition base=200000:.../canonical-cxsmiles-opt/image-only/
                              public-add-mp-canonical-4e6cb96/train.jsonl \
    --partition hard=50000:.../targeted-replay/
                              sft2b_ckpt16000_hardslice_50k_seed74/train.jsonl \
    --output-jsonl  .../no-synthetic-250k-seed74-80base-20hard/train.jsonl \
    --manifest-json .../no-synthetic-250k-seed74-80base-20hard/manifest.json \
    --seed 74 --require-absolute-images
Manifest: no-synthetic-250k-seed74-80base-20hard/manifest.json
  written_rows           : 250000
  partition_counts       : base 200000, hard 50000
  source_counts          : mg1_synthetic 152620, uspto_mol_m 52524, molparser 44856
  mode_counts            : patent_image_markush 152620,
                           structure_only_markush 52524,
                           molparser_converted_markush 44856
  target_format_counts   : "canonicalized cxsmiles_opt" 250000
  target_canon_status    : already_canonical 155415, canonicalized 94585
\end{verbatim}
\end{footnotesize}
\end{figure}

\subsection{OCSR-as-Markush mixtures and decontamination}
\label{app:repro_ocsr_mix}

The three ordinary-molecule fractions are built from the MolScribe OCSR pool,
converted to no-extension Markush records, and decontaminated against the
ordinary-molecule OCSR evaluation sets. The ordinary count at fraction $f$ is
$\mathrm{round}\!\left(\tfrac{f}{1-f}\times 250000\right)$.

\begin{table}[tb]
    \centering
    \small
    \caption{OCSR-as-Markush mixtures over the fixed 250{,}000-row Markush base.
    Every value is read from the corresponding
    \texttt{ocsr-fraction-\{5,10,15\}pct-seed74-decontam/manifest.json}; the
    eval-overlap removal count and the post-decontamination overlap are quoted
    from \texttt{decontamination\_removed\_count} and
    \texttt{post\_decontamination\_leakage\_check.overlap\_rows}.}
    \label{tab:repro_ocsr_mix}
    \begin{tabularx}{\linewidth}{@{}l r r r r@{}}
        \toprule
        Fraction & Ordinary rows & Total rows & Removed (eval overlap) & Post-decon. overlap \\
        \midrule
        5\%  & 13{,}158 & 263{,}158 & 80 & 0 \\
        10\% & 27{,}778 & 277{,}778 & 80 & 0 \\
        15\% & 44{,}118 & 294{,}118 & 80 & 0 \\
        \bottomrule
    \end{tabularx}

    \vspace{0.4em}
    \parbox{\linewidth}{\raggedright\footnotesize
    % ocsr_count / total_rows / decontamination_removed_count /
    % post_decontamination_leakage_check.overlap_rows per manifest;
    % cross-checked in ocsr-fraction-decontam-summary-seed74.json (all overlap 0).
    Pool: \texttt{molscribe-ocsr/.../unified.jsonl}, 680{,}220 source rows;
    680{,}140 trainable; 625{,}089 eligible after decontamination. Evaluation
    reference: 12{,}870 rows / 11{,}259 unique canonical SMILES across CLEF, JPO,
    UOB, USPTO. Eligibility is an RDKit-canonical-SMILES match against that
    reference; no-extension target is
    \texttt{<markush><cxsmi>SMILES</cxsmi><stable></stable></markush>}.}
\end{table}

\begin{figure}[tbp]
\begin{footnotesize}
\begin{verbatim}
=== Listing: OCSR-as-Markush decontaminated mixes ===
Builder: scripts/prepare_final_multitask_sft.py   (autoresearch-markush)
  no-extension conversion: ocsr_row_as_no_extension_markush(...)
    target = "<markush><cxsmi>{canonical_smiles}</cxsmi><stable></stable></markush>"
  ordinary count: round(frac / (1 - frac) * 250000)
    f=0.05 -> 13158 ; f=0.10 -> 27778 ; f=0.15 -> 44118   (reproduced exactly)
Source pool (manifest decontamination.source_jsonl):
  .../ocsr-markush-multitask/imports_20260616_7cb5bc9/molscribe-ocsr/unified.jsonl
  source_rows 680220 ; trainable_kept_rows 680140 ; eligible 625089
Eval reference (manifest ocsr_eval_canonical_smiles):
  .../eval/ocsr-as-markush-no-extension-20260625/eval_ocsr_{clef,jpo,uob,uspto}.jsonl
  rows 12870 ; unique_canonical_smiles 11259 ; invalid_rows 0
Per-fraction manifests record:
  decontamination_removed_count = 80   (all three)
  post_decontamination_leakage_check.overlap_rows = 0, severity "none" (all three)
\end{verbatim}
\end{footnotesize}
\end{figure}

\subsection{Synthetic Markush-rendering mixtures}
\label{app:repro_synth_mix}

\begin{figure}[tbp]
\begin{footnotesize}
\begin{verbatim}
=== Listing: synthetic-mix mixtures (under re-test; no outcome asserted) ===
Builder: scripts/build_stable_scaling_sft_mix.py   (autoresearch-markush)
Synthetic pool: PubChem-scaffold pool -> markush.data.pipeline eval_aligned
  decoration -> MarkushGenerator render (train-like, structure_only)
synthetic-mix-260k-seed74/manifest.json:
  command base=250000:.../no-synthetic-250k-seed74-80base-20hard/train.jsonl
          synth=10000:.../synthetic-rendered/existing-eval-like-10k-1a4f16a/train.jsonl
  written_rows 260000 ; synth selected_count 10000 (eligible 9473)
  synth share of mix = 10000/260000 = 3.8%
synthetic-mix-350k-seed74/manifest.json:
  command base=250000:... synth=100000:.../existing-eval-like-100k-1a4f16a/train.jsonl
  written_rows 350000 ; synth selected_count 100000 (eligible 60388)
  synth share of mix = 100000/350000 = 28.6%
Leakage: synthetic-mix-leakage-check-seed74.json
  eval set = public-markush-full-1055 (IP5-M + M2S + USPTO-Markush), eval_rows 1055
  both pools: overlap_rows 0, overlap_fraction 0.0, severity "none"
\end{verbatim}
\end{footnotesize}
\end{figure}

\subsection{Dedicated OCSR training data}
\label{app:repro_ocsr_data}

The dedicated OCSR model is trained from scratch (ImageNet vision backbone
allowed; no OCSR-specific pretrained checkpoints). The best checkpoint is
\texttt{v8-3} at canonical exact match 0.9397 (5{,}360/5{,}704), recipe in
\texttt{checkpoints/v8-3-recipe.json}. Molecule sources come from the public
mirror \texttt{CYF200127/MolNexTR}. Because the rendered training data was not
retained, the inputs are re-derived from the cached/curated sources rather than
restored verbatim.

\begin{figure}[tbp]
\begin{footnotesize}
\begin{verbatim}
=== Listing: dedicated OCSR training inputs (v8-3 headline recipe) ===
Launch (recorded in campaigns/ocsr/v10/{launch_main,direct_launch,run_continue}.sh):
  python -m torch.distributed.run --standalone --nproc_per_node=8 \
    -m autoresearch.train \
    --pubchem_csv       .../raw/train_pubchem.csv         # PubChem-1M, Indigo on-the-fly
    --uspto_csv         .../uspto_mol/train_uspto.csv \
    --uspto_image_root  .../uspto_mol/train_uspto \       # USPTO-680k, pre-rendered TIFs
    --uspto_path_strip_prefix uspto_mol/ \
    --extra_pubchem_csv .../canary_similar_pubchem.csv  --extra_pubchem_repeat 2 \
    --stereo_csv        .../stereo_200k_white/train.csv --stereo_repeat 2 \
    --backbone_pretrained --cosine_lr --augment_v2 --bf16_amp ...
Inputs and row counts:
  PubChem-1M               train_pubchem.csv            1,000,000  (Indigo, dynamic)
  USPTO-680k               train_uspto.csv                680,220  (pre-rendered)
  stereo_200k_white        stereo_200k_white/train.csv    200,000  x2
  canary_similar_pubchem   canary_similar_pubchem.csv      64,752  x2
Effective dataset_size = 1,000,000 + 680,220 + 2*200,000 + 2*64,752 = 2,209,724
  (matches dataset_size=2209724 in the v8-3 train.log and v8-2-analysis.json)
Recipe (checkpoints/v8-3-recipe.json):
  encoder swin_base_patch4_window12_384 (ImageNet) + 6-layer transformer decoder
  target_format chartok_smiles_only (RDKit-canonical SMILES); seed 42
  primary_recipe MolNexTR; ocsr_specific_pretrained_checkpoints_forbidden true
Re-derivation: PubChem-1M served from the cached train_pubchem.csv (no re-download);
  stereo + canary curated CSVs preserved on disk under datasets-curated/v6-fresh/
  (regenerate-free); USPTO images re-rendered from train_uspto.zip.
\end{verbatim}
\end{footnotesize}
\end{figure}

%% DISCREPANCY (blocking; resolve before merge): the task brief described the
%% four OCSR inputs as PubChem-1M + USPTO-680k + "stereo-curriculum (50,336,
%% oversampled x20)" + "canary RDKit (50,336)", assembled by prepare_data.py.
%% The VERIFIED v8-3 headline recipe (above) instead uses stereo_200k_white
%% (200,000, x2) + canary_similar_pubchem (64,752, x2), launched via
%% `autoresearch.train` (no prepare_data.py found on disk). The "50k stereo-rich
%% molecules x20 oversampling" phrasing is real but belongs to an EARLIER v7
%% iteration (notes/v7_summary.json "Scratch_stereo_enriched..."), not v8-3.
%% Files stereo_curriculum_v2.csv and canary_rdkit_training.csv (both 50,336
%% lines incl. header) exist under datasets-curated/v6-fresh/ but are not the
%% v8-3 inputs. I report only what the v8-3 run records support.

%% ----------------------------------------------------------------------------
%% SHA256 / pin status
%% ----------------------------------------------------------------------------
\paragraph{Artifact pins.}
Each Markush mixture is pinned by its \texttt{manifest.json} (seed, exact
partition paths, per-source counts, target-conversion counts, decontamination
results) and the corresponding \texttt{report.md}. The synthetic-rendered pools
carry a content tag in their directory name
(\texttt{existing-eval-like-\{10k,100k\}-1a4f16a}), and the
synthetic-augmented variants pin a git-style hash
(\texttt{...-892e1dd} for the 260k arm, \texttt{...-966041b} for the 350k arm).
The OCSR molecule sources are pinned by the HF dataset id
\texttt{CYF200127/MolNexTR} and the recorded row counts
(\texttt{train\_pubchem.csv} 1{,}000{,}000; \texttt{train\_uspto.csv}
680{,}220).
%% UNVERIFIED: no explicit per-file SHA256 hashes were found in the manifests
%% for the training mixes. The manifests pin by exact path + row/source counts +
%% seed, and the synthetic dirs carry short content/commit tags (1a4f16a /
%% 892e1dd / 966041b), but a true sha256 digest field was not present in any
%% manifest read. The OCSR eval contract (notes/eval_contract.md) is described
%% as sha256-locked on (id-sorted) and (canonical-SMILES-sorted) hashes, but the
%% digest VALUES were not read in this pass. If the paper needs literal SHA256
%% strings, point me at the file(s) holding them.
